# Supplementary material for: High-Throughput GW Calculations via Machine Learning
Source: arXiv:2505.02421 source file (2025-05-05)
Supplement: Supplementary file 1 [file supplemental_material.pdf]

# Supplemental Material: High-Throughput GW Calculations via Machine Learning

R. A. Abdelghany
*Physics Department, Faculty of Science, Al-Azhar University, Assiut, 71524, Egypt and*
*Department of Physics, National Chung Hsing University, Taichung, 40227, Taiwan*

Chih-En Hsu and Hung-Chung Hsueh
*Department of Physics, Tamkang University, New Taipei 251301, Taiwan*

Yuan-Hong Tsai
*AI Foundation, Taipei, 110, Taiwan*

Ming-Chiang Chung*
*Department of Physics, National Chung Hsing University, Taichung, 40227, Taiwan*
*Physics Division, National Center for Theoretical Sciences, Taipei, 10617, Taiwan and*
*Max Planck Institute for the Physics of Complex Systems,*
*Nöthnitzer Straße 38, Dresden, 01187, Germany*

(Dated: May 5, 2025)

PACS numbers:

## I AB INITIO CALCULATIONS

Molecular Dynamics (MD) simulations were employed to generate datasets for training, validation, and testing the model. These simulations were performed using the Quantum Espresso package[1–3], employing a variable-cell Car-Parrinello (vc-cp) approach to allow for both atomic and cell relaxation. The simulations were propagated for 5000 time steps, with an integration time step (dt) of 5.0 a.u.. A plane-wave energy cutoff of 70 Ry was used to ensure an accurate representation of the electronic wavefunctions. The atomic positions were randomized with an amplitude of 0.2 a.u. to ensure proper sampling of the configuration space. The simulations were coupled with a Nosé-Hoover thermostat to maintain the ion temperature at 300 K. From the ensemble of generated configurations for each BN polymorph, 1000 snapshots were selected for subsequent GW calculations. These snapshots were chosen at evenly spaced intervals throughout the entire simulation trajectory to ensure a representative sampling of the dynamic structural fluctuations and to capture the range of atomic configurations explored during the MD simulation.

By simulating different structures using MD at finite temperatures, we account for thermal fluctuations that induce atomic displacements and transient electronic structure modifications. These structural variations lead to changes in the quasiparticle energies, including band gap shrinkage or even collapse to zero in certain MD snapshots—a phenomenon consistent with dynamic metallization under thermal, strain, or excitation conditions. Such behavior has been observed in previous studies, where MD coupled with electronic structure calculations successfully captured band gap reduction and transient metallization due to structural distortions. By incorporating these diverse configurations into our training dataset, the machine learning model can better generalize across different electronic regimes, enhancing its predictive accuracy for insulating and metallic phases[4–13].

Ab initio Density Functional Theory (DFT) calculations were conducted using Quantum ESPRESSO, and GW calculations were performed with BerkeleyGW[14,15]. Randomly selected snapshots confirmed that mean-field calculations achieved convergence using k-point sampling via the Monkhorst-Pack method with an 8x8x8 grid (512 k-points). GW calculations require including a large number of unoccupied bands in the mean-field calculations, which poses a significant computational challenge, especially for multiple MD snapshots. In this work, reasonable convergence was obtained by considering 150 Kohn-Sham bands. The different structures considered in this study are shown in Fig. (1).

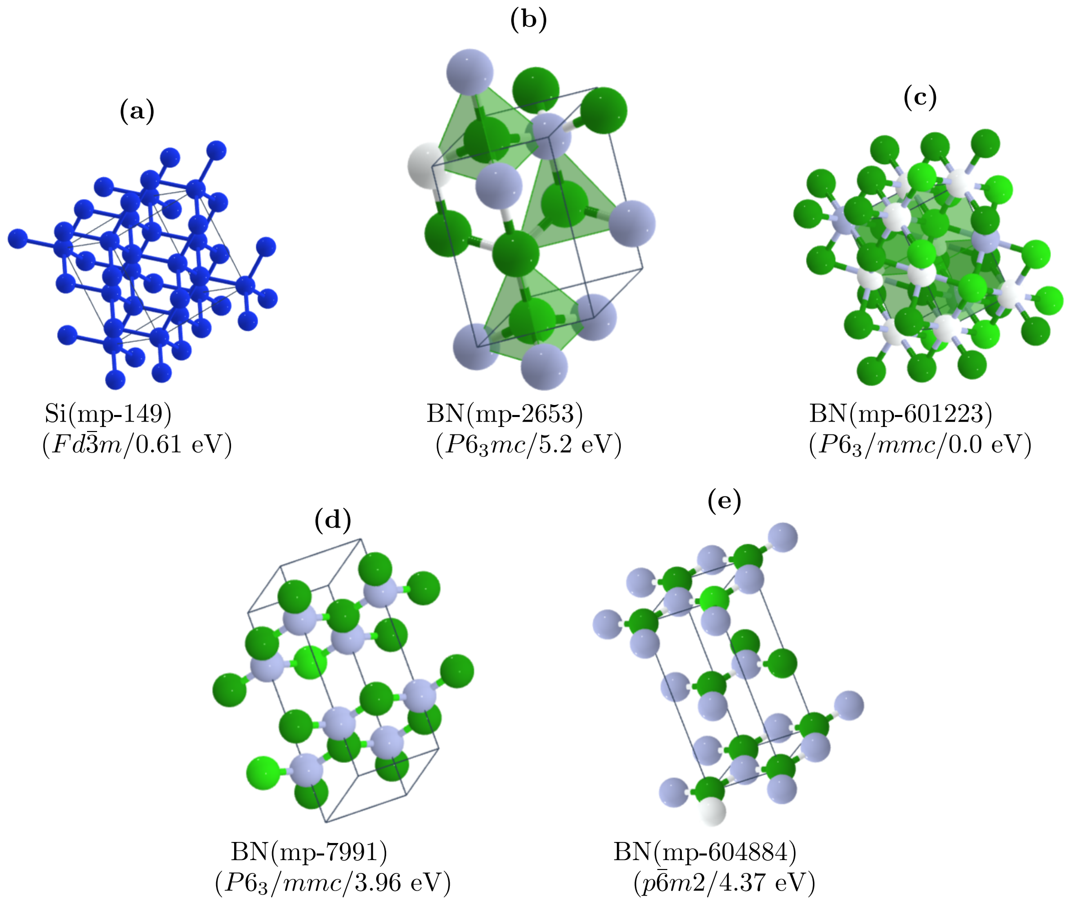


FIG. 1: Crystal structures and electronic properties of Si and BN polymorphs. Space groups and band gaps (in eV, from DFT) are denoted in parentheses for each structure. Structures are visualized from the Materials Project database[16].

## II MACHINE LEARNING MODEL

We employed a gradient-boosting machine learning model, specifically a LightGBM regressor[17], to predict GW quasiparticle energies ($E_{QP}$) using mean-field energies ($E_{MF}$) and the exchange-correlation potential ($V_{XC}$) as input features. The model was implemented using the LightGBM framework, which is optimized for efficiency and scalability, particularly for large datasets. The training process was designed to capture the nonlinear relationship between the input features and the target quasiparticle energies.

### A. Input Features and Preprocessing

The input features for the model were constructed from the mean-field energies and the exchange-correlation potential. To enhance the model's ability to capture nonlinear relationships, we included higher-order terms and logarithmic transformations of the input features. Specifically, the feature vector for each data point was constructed as follows:

$$\mathbf{X} = \left[V_{\mathrm{MF}}, E_{\mathrm{XC}}, E_{\mathrm{MF}}^2, V_{\mathrm{XC}}^2, E_{\mathrm{MF}}^3, V_{\mathrm{XC}}^3, \log(1+|V_{\mathrm{MF}}|), \log(1+|E_{\mathrm{XC}}|), \log(1+|E_{\mathrm{MF}} \cdot V_{\mathrm{XC}}|)\right], \tag{1}$$

Here, $E_{MF}$ and $V_{XC}$ are matrices of size $N \times B$, where $N$ is the number of snapshots and $B$ is the number of bands considered. The logarithmic transformations ($\log(1+|x|)$) were applied to ensure numerical stability and to capture the scaling behavior of the input features. To ensure consistent scaling across features and targets, the input features ($\mathbf{X}$) and target quasiparticle energies ($E_{QP}$) were normalized using the MinMaxScaler from the scikit-learn library.

### B. Hyperparameter Optimization and Training

The LightGBM regressor was configured with the following hyperparameters, which were optimized using the Optuna framework[18]:

- Boosting type: Gradient Boosting Decision Trees (GBDT)
- Objective function: Regression (mean squared error)
- Number of leaves: 69
- Learning rate: 0.0201
- Number of estimators: 6781
- Device: GPU (for accelerated training)

The model was trained using a multi-output regression approach, implemented via the MultiOutputRegressor wrapper in scikit-learn, to simultaneously predict quasiparticle energies for all bands.

### C. Loss Function and Evaluation Metrics

The model was trained to minimize the mean squared error (MSE) between the predicted and actual quasiparticle energies:

$$\text{MSE} = \frac{1}{N} \sum_{i=1}^{N} \left( E_{\text{QP, predicted}}^{(i)} - E_{\text{QP, actual}}^{(i)} \right)^2 \tag{2}$$

$$R^2 = 1 - \frac{\sum_{i=1}^{N} \left( E_{\text{QP, predicted}}^{(i)} - E_{\text{QP, actual}}^{(i)} \right)^2}{\sum_{i=1}^{N} \left( E_{\text{QP, actual}}^{(i)} - \bar{E}_{\text{QP, actual}} \right)^2} \tag{3}$$

Here, $\bar{E}_{\text{QP, actual}}$ is the mean of the actual quasiparticle energies.

## III Model Evaluation

The parity plot (2) compares the predicted quasiparticle energies ($E_{nk}^{ML}$) against the actual quasiparticle energies ($E_{nk}^{GW}$) for BN (mp-2653). As shown in Fig. 2(a), the predictions lie very close to the $y = x$ line, indicating excellent agreement between the predicted and actual values. The model achieves $R^2$ of 1 and RMSE of 0.0239 eV, demonstrating its high predictive accuracy. The near-perfect alignment of the data points with the $y = x$ line confirms that the model captures the underlying physical relationships between the input features (mean-field energies and exchange-correlation potential) and the target quasiparticle energies.

The difference histogram illustrates the distribution of residuals, defined as the difference between the predicted and actual quasiparticle energies ($E_{nk}^{GW} - E_{nk}^{ML}$). As shown in Fig. 2(b), the residuals for both the training and validation sets are narrowly peaked, symmetric, and centered around zero. This indicates that the model's errors are minimal and randomly distributed, with no systematic bias. The similarity in the distributions of the training and validation sets further confirms that the model generalizes well to unseen data, with no signs of overfitting.

The training process involved 100 iterations, with the data shuffled at the beginning of each iteration to ensure robust learning. The dataset was split into training and validation sets (80:20 ratio) at each iteration to monitor the model's performance and prevent overfitting. All 100 iterations of the model training yielded similar performance metrics, with an average $R^2$ of 1 and an average RMSE of 0.025 eV. This consistency across iterations underscores the robustness and reliability of the model. The small variation in RMSE and the consistently high $R^2$ values indicate that the model is stable and not sensitive to the random initialization of data shuffling or training-validation splits.

To systematically examine the correlation between model performance and the size of the training dataset, $R^2$ and mean squared error (MSE) were evaluated for the hold-out dataset as a function of the percentage of data utilized for training, as illustrated in Fig. 3. As shown in the figure, the $R^2$ value increases rapidly with the training data size, reaching a plateau beyond approximately 25%. Conversely, the MSE exhibits an inverse trend, decreasing from 0.176 eV when the training data is at its smallest size (7%) and continuing to decrease as the training dataset expands.

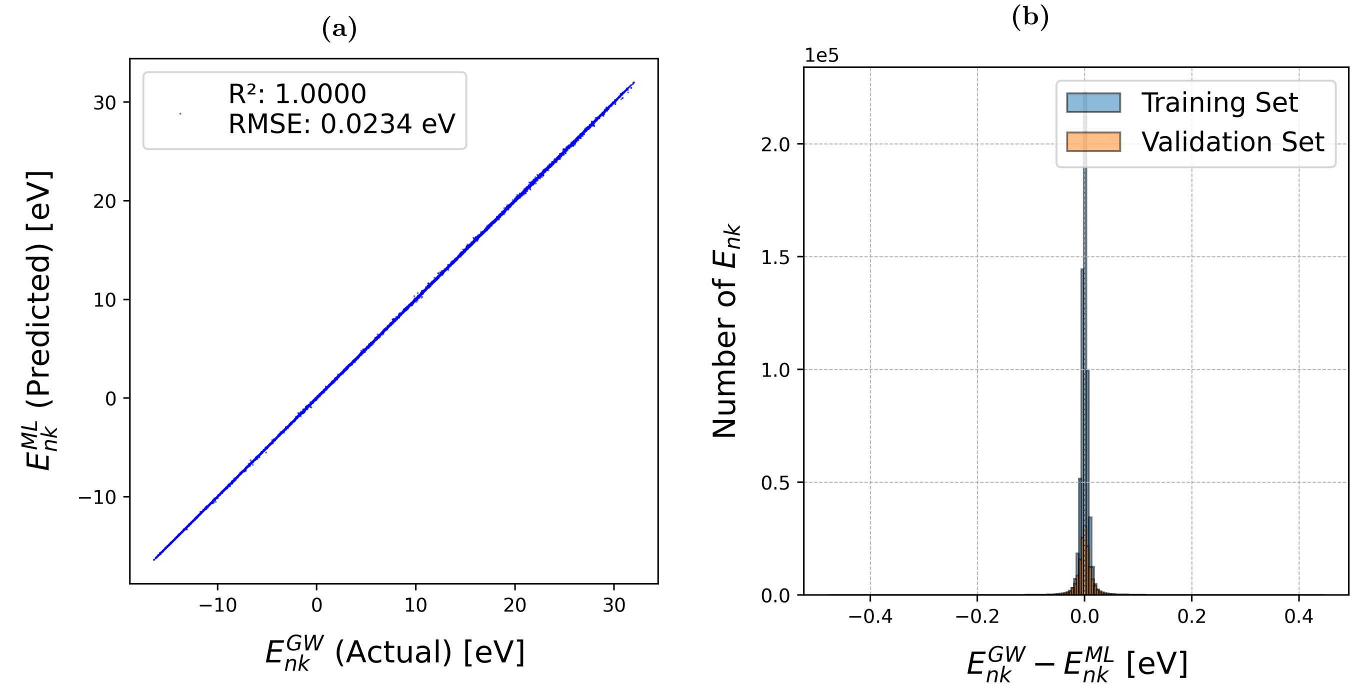


FIG. 2: Model evaluation for an arbitrarily chosen iteration: (a) Parity plot comparing predicted and actual quasiparticle energies, showing excellent agreement with $R^2 \approx 1$ and RMSE = 0.0239 eV. (b) Histogram of residuals (predicted − actual) for the training and validation sets, demonstrating narrowly peaked, symmetric distributions centered around zero, indicating minimal and unbiased errors.

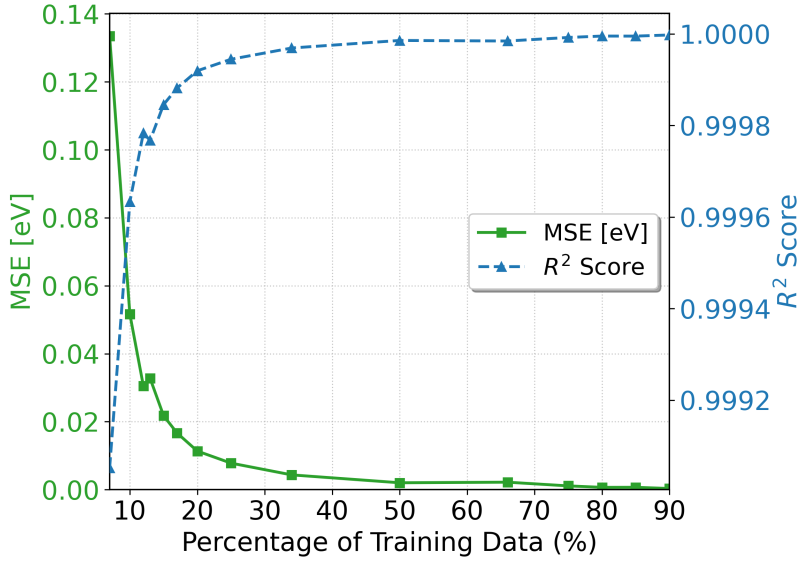


FIG. 3: Model performance metrics, $R^2$ and MSE, as a function of the percentage of training data used. Performance is evaluated on the data not included in the training sets.

## IV Training different BN structures

We followed the same training strategy as in the main analysis, using 25% of the MD snapshots for training and validation, and the remaining 75% for testing. In this section, we applied this approach to three different BN crystal structures: BN(mp-2653), BN(mp-601223), and BN(mp-7991), each with distinct space groups and band gaps, as illustrated in Fig. (1).

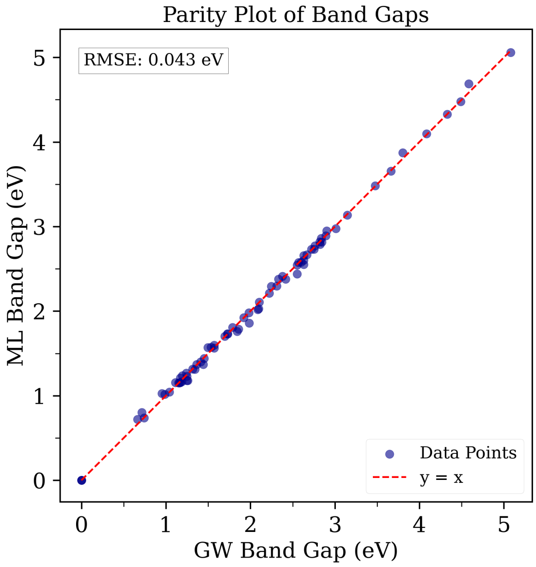


FIG. 4: Parity plot comparing ML-predicted and GW-calculated band gaps for BN(mp-7991) snapshots excluded from training. The close alignment along the $y = x$ line and the low RMSE value of 0.043 eV indicate strong predictive accuracy of the ML model.

The parity plot shown in Fig. (4) presents the comparison between the ML and GW-calculated band gaps for BN(mp-7991) snapshots not included in the training process. The RMSE between the predicted and reference values is 0.043 eV, demonstrating excellent agreement between the ML predictions and the GW results.

To further assess the predictive performance of the ML model, we present the density of states (DOS) for four arbitrarily selected BN(mp-7991) snapshots, comparing the ML-predicted DOS (red solid lines) with the reference GW-calculated DOS (blue dashed lines). As shown in Fig. (5), the ML model accurately reproduces the DOS profiles across the entire energy spectrum, despite the distinct spectral features exhibited by different snapshots. The energy difference between the ML and GW band gaps, defined as $\Delta E = E_{\mathrm{ML}} - E_{\mathrm{GW}}$, remains small for all cases: -0.019 eV (Snapshot 1), -0.017 eV (Snapshot 19), -0.028 eV (Snapshot 75), and 0.000 eV (Snapshot 41). These results confirm the model's robustness and generalization capability in capturing both qualitative and quantitative aspects of the electronic structure under thermal fluctuations.

---

* Electronic address: `mingchiangha@nchu.edu.tw`

[1] P. Giannozzi et al., QUANTUM ESPRESSO: a modular and open-source software project for quantum simulations of materials, *J. Phys.: Condens. Matter* **21**, 395502 (2009).
[2] P. Giannozzi et al., Advanced capabilities for materials modelling with Quantum ESPRESSO, *J. Phys.: Condens. Matter* **29**, 465901 (2017).
[3] P. Giannozzi et al., Quantum ESPRESSO toward the exascale, *J. Chem. Phys.* **152**, 154105 (2020).
[4] Y. Zhang, C. Wang, F. Zheng, and P. Zhang, Quantum molecular dynamics simulations for the nonmetal-metal transition in fluid nitrogen oxide, *J. Appl. Phys.* **112**, 033503 (2012).
[5] S. Liu, B. Liu, X. Shi, J. Lv, S. Niu, M. Yao, Q. Li, R. Liu, T. Cui, and B. Liu, Two-dimensional penta-BP5 sheets: High-stability, strain-tunable electronic structure and excellent mechanical properties, *Sci. Rep.* **7**, 2404 (2017).
[6] K. Takai, M. Ikeda, T. Yamasaki, and C. Kaneta, Size and temperature dependence of the energy gaps in Si, SiC and C quantum dots based on tight-binding molecular dynamics simulations, *J. Phys. Commun.* **1**, 045010 (2017).
[7] Y.-L. Lu, S. Dong, W. Zhou, S. Dai, B. Zhou, H. Zhao, and P. Wu, Hittorf's violet phosphorene as a promising candidate for optoelectronic and photocatalytic applications: first-principles characterization, *Phys. Chem. Chem. Phys.* **20**, 11967 (2018).
[8] H.-Y. Ye, F.-F. Hu, H.-Y. Tang, L.-W. Yang, X.-P. Chen, L.-G. Wang, and G.-Q. Zhang, Germanene on single-layer ZnSe substrate: novel electronic and optical properties, *Phys. Chem. Chem. Phys.* **20**, 16067 (2018).
[9] K. Konstantinou, T.-H. Lee, F. C. Mocanu, and S. R. Elliott, Origin of radiation tolerance in amorphous Ge2Sb2Te5 phase-change random-access memory material, *Proc. Natl. Acad. Sci.* **115**, 5353 (2018).
[10] A. Mei and X. Luo, The structural, electronic and optical properties of $\gamma$-glycine under pressure: a first principles study,

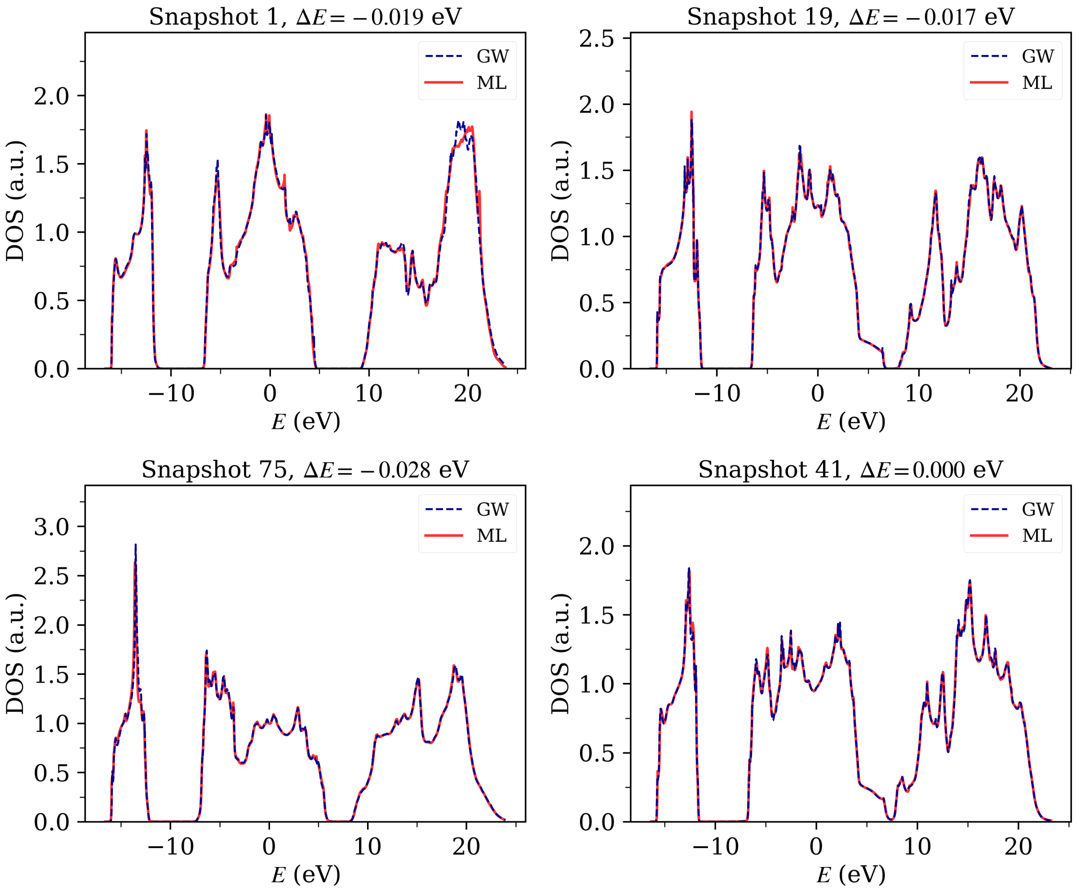


FIG. 5: Comparison of DOS for four selected BN(mp-7991) snapshots. The ML-predicted DOS (red solid lines) closely match the GW-calculated DOS (blue dashed lines) across the full energy range. The small band gap deviations $\Delta E$ further demonstrate the model's reliability in capturing thermal-induced electronic structure variations.


*RSC Adv.* **9**, 3877 (2019).

[11] L. C. Nhan, V. T. T. Vi, D. X. Du, N. Q. Cuong, N. N. Hieu, and T. P. T. Linh, Density functional theory investigations of PbSnX2 (X= S, Se, Te) monolayers: Structural and electronic properties, *Chem. Phys.* **566**, 111797 (2023).

[12] H. Dong, J. Zhao, H. Yang, and Y. Zheng, Tunable long-lived exciton lifetime in single-layer two-dimensional $LiAlTe_2$, *Phys. Rev. Mater.* **6**, 104001 (2022).

[13] J. Hu, Y. Li, X. Quan, and T. Ma, Molecular dynamics simulations on TiO2 quantum dots modified asphalt: Impact of size and concentration of quantum dots, *Comput. Theor. Chem.* **1238**, 114726 (2024).

[14] M. S. Hybertsen and S. G. Louie, Electron correlation in semiconductors and insulators: Band gaps and quasiparticle energies, *Phys. Rev. B* **34**, 5390 (1986).

[15] J. Deslippe et al., BerkeleyGW: A massively parallel computer package for the calculation of the quasiparticle and optical properties of materials and nanostructures, *Comput. Phys. Commun.* **183**, 1269 (2012).

[16] A. Jain et al., Commentary: The Materials Project: A materials genome approach to accelerating materials innovation, *APL Mater.* **1**, 011002 (2013).

[17] G. Ke, Q. Meng, T. Finley, T. Wang, W. Chen, W. Ma, Q. Ye, and T.-Y. Liu, LightGBM: A highly efficient gradient boosting decision tree, *Adv. Neural Inf. Process. Syst.* **30** (2017).

[18] T. Akiba, S. Sano, T. Yanase, T. Ohta, and M. Koyama, Optuna: A next-generation hyperparameter optimization framework, in *Proc. 25th ACM SIGKDD Int. Conf. Knowl. Discov. Data Min.*, p. 2623 (2019).
